# Supplementary material for: Language-Conditioned Imitation Learning with Base Skill Priors under Unstructured Data
Source: arXiv:2305.19075 source file (2024-09-12)
Supplement: Supplementary file 1 [file 09_appendix.tex]

\section{Terminology}
\begin{table}[htbp]
    \centering
    \caption{Terminology}
    % \resizebox{0.48\textwidth}{!}{
    \begin{tabular}{ l l }
        \toprule
        Notations & Definition \\
        \midrule
        $\mathcal{S}$ & State space \\
        $\mathcal{A}$ & Action space \\
        $\mathcal{A}_\textrm{skill}$ & Skill space  \\
        $\mathcal{A}_z$ & Skill embedding space \\
        $\mathcal{P}$ & Environment dynamics \\
        $\mathcal{G}$ & Multi-context goal space \\
        $\mathcal{I}$ & Language instruction set\\
        $x$ & Action sequence $(a_0, a_1, ...)$\\
        $y$ & Base skills, $y \in \{\textrm{translation}, \textrm{rotation}, \textrm{grasping}\}$\\
        $z$ & Skill embedding in the latent space \\
        $N_h$ & Horizon of action sequence (skill) \\
        $N_o$ & Number of observations \\
        $N_z$ & Skill embedding dimension\\
        $f_{\boldsymbol{\kappa}}$ & Base skill locator network with parameters $\boldsymbol{\kappa}$\\
        $f_{\boldsymbol{\theta}}$ & Skill generator network with parameters $\boldsymbol{\theta}$\\
        $f_{\boldsymbol{\phi}}$ & Encoder network for action sequences\\
        
        $f_{\boldsymbol{\Phi}}$ & Encoder network of our SPIL model\\
        $f_{\boldsymbol{\lambda}}$ & Skill embedding selector network with parameters $\boldsymbol{\lambda}$ \\
        $f_{\boldsymbol{\omega}}$& Base skill selector network with parameters $\boldsymbol{\omega}$\\
        
        \bottomrule
    \end{tabular}
    % }
    \label{tab:terminology}
\end{table}

\section{Problem Statement}
\label{sec:problem statement}
Our methods aim to learn a goal-conditioned policy $\pi(a|s,l)$ that outputs action $a \in \mathcal{A}$, conditioned on the current state $s \in \mathcal{S}$ and a language instruction $l \in \mathcal{I}$, under environment dynamics $\mathcal{P}: \mathcal{S} \times \mathcal{A} \rightarrow \mathcal{S}$. The environment can be characterized by the following statements:
\begin{itemize}
    \item A multidimensional action space $\mathcal{A} \subset \mathbb{R}^7$. This actions space contains all parameters to drive the agent to finish tasks. The first three parameters are the displacement of the end-effector's position. Another three parameters are the rotation of the end effector and the final parameters is the gripper control parameters.
    \item A visual state $\mathcal{S} \subset \mathbb{R}^{N_o \times H \times W \times 3}$, where $N_o$ is the number of observations. H and W are the height and width of the images. 3 is the channel numbers since the agent only has access to visual observations from cameras.
    \item A multi-context goal space consists of language instructions and goal images $\mathcal{G} \subset \mathcal{I} \cup \mathbb{R}^{H \times W \times 3}$, where $\mathcal{I}$ is the nature language set and $H$, $W$ are the height and width of images, respectively. 
\end{itemize}

\section{CALVIN Environment Detail}
\label{sec:CALVIN Environment Detail}
Mees et al. introduce the CALVIN benchmark \cite{mees2022calvin} to facilitate learning language-conditioned tasks across four manipulation environments. We mainly use this benchmark to evaluate our SPIL model's performance. CALVIN benchmark mainly contains three components.
\begin{itemize}
    \item \textbf{CALVIN environments}. CALVIN includes four distinct environments (A, B, C, D) that are interconnected in terms of their underlying structure. Each environment consists of one Franka Emika Panda robot arm equipped with a gripper and a desk featuring a sliding door and a drawer that can be opened and closed. On the desk, there exists a button that can toggle the green light and a switch to control a light bulb. Note that each environment has a different desk with various of textures and the position of static elements such as the sliding door, drawer, light, switch, and button are different across each environment. 
    \item \textbf{CALVIN dataset}. To comprehensively explore the possible scenarios within a given space, the individuals involved engaged in teleoperated play while wearing an HTC Vive VR headset for a total of 24 hours, spending roughly the same amount of time (6 hours) in each of four different environments. In terms of language instructions, they utilize 400 natural language instructions that correspond to over 34 different tasks to label episodes in a procedural manner, based on the recorded state of the environment in the CALVIN dataset.
    \item \textbf{CALVIN challenge}. The authors of the CALVIN introduce various evaluation protocols and metrics of different difficulty levels. These protocols are
        \begin{itemize}
            \item \textbf{Single Environment:} Training in a single environment and evaluating the policy in the same environment.
            \item \textbf{Multi Environment:} Training in all four environments and evaluating the policy in one of them. 
            \item \textbf{Zero-Shot Multi Environment:} This involves training the agent in three different environments and then testing its ability to generalize and perform well in a fourth environment that it has not previously encountered.
        \end{itemize}
    and the metrics are 
    \begin{itemize}
        \item \textbf{Multi-Task Language Control (MTLC):} The most straightforward evaluation aims to verify how well the learned multi-task language-conditioned policy generalizes 34 manipulation tasks
        \item \textbf{Long-Horizon Multi-Task Language Control (LH-MTLC):} In this evaluation, the 34 tasks from a previous evaluation are treated as subgoals, and valid sequences consisting of five sequential tasks are computed.
    \end{itemize}
\end{itemize}

\section{Comparison with Other Skill-based Approaches}
\label{sec:Comparison with Other Skill-based Approaches}
To showcase our model's exceptional performance relative to other skill-based reinforcement learning approaches, we've adapted the CALVIN benchmark to match the assessment criteria utilized in those approaches. This modified benchmark focuses on a subset of tasks within the CALVIN benchmark for evaluation purposes. The baselines we choose are two skill-based reinforcement learning approaches SpiRL \cite{shiskill} and SkiMo \cite{pertsch2020spirl}. We assess these methods using a fixed task chain comprising four assignments, namely Open Drawer - Turn on Lightbulb - Move Slider Left - Turn on LED. This task sequence is evaluated 1000 times to determine the average success rate. The outcomes are presented in Table \ref{tab:skill-based approach comparisons}. Our SPIL approach consistently attains an almost perfect success rate of nearly 100\% in this task sequence, outperforming the other baseline methods that utilize skill-based reinforcement learning for agent training. All experiments are evaluated with 3 random seeds. 
\begin{table}[h]
  \caption{Skill-based approaches}\label{tab:skill-based approach comparisons}
  \centering
  \resizebox{.48\textwidth}{!}{
  \begin{tabular}{l l l l}
    \hline
      Model & SpiRL & SkiMO & SPIL(ours) \\
    \hline
      Avg. Len. (\#/4.00) & $3.02 (0.53)$ & $3.64 (0.21)$ & $\textbf{3.99} (0.01)$ \\
    \hline
  \end{tabular}
  }
\end{table}
\section{Implementation Details}
\subsection{Skill Embedding Space Generation}
For the Single Environment, the skill embedding space is generated by the action sequences in the training data of environment D. Regarding to Zero-shot Multi Environment, the skill embedding space is generated by the action sequences in the training data of environment A, B, and C. Important hyperparameters are listed in Table \ref{table: important hyperparameters (Single Environment)} and \ref{table: important hyperparameters (Zero-shot Multi Environment)}.

\subsection{Training Setting}
The hyperparameters leveraged to train the agent in Single Environment and Zero-shot Multi Environment settings are listed in Table \ref{table: important hyperparameters (Single Environment)} and \ref{table: important hyperparameters (Zero-shot Multi Environment)}. The camera observations are applied with an image augmentation strategy. For simulation evaluations, the static observation goes through random shift of 10 pixels and normalization with mean=[0.48145466, 0.4578275, 0.40821073] and std=[0.26862954, 0.26130258, 0.27577711]; the gripper observation goes through random shift of 4 pixels and normalization with the same mean and std as static observation;

For real-world experiments, we apply stronger augmentation for images. The static observation goes through the following transforms, random shift of 10 pixels, color jitter with 0.2 brightness and 0.2 contrast, random rotation with the range of (-5, 5) degrees, random perspective with distortion-scale 0.1, and finally normalization with mean=[0.48145466, 0.4578275, 0.40821073] and std=[0.26862954, 0.26130258, 0.27577711]. The gripper observation goes through center cropping, random shift with 4 pixels, color jitter with 0.2 brightness and 0.2 contrast, and finally the same normalization as the static observation. 

We have also implemented an augmentation strategy for action sequences during the skill embedding training, where we randomly set the last three relative actions of a sequence to zero, indicating still actions.

\begin{table}[ht]
    \centering
    \caption{Important hyperparameters (Single Environment)}
       \label{table: important hyperparameters (Single Environment)}
    \resizebox{.4\textwidth}{!}{
    \begin{tabular}{ c | c} 
        \hline
            Description & Value \\
        \hline
            Batch Size & 64 \\
            Learning Rate &  $1.0 \times 10^{-4}$  \\ 
            Skill Embedding Dimension & 20 \\
            Horizon Length $H$ of Skill & 5 \\
            Magic Scales $w_1, w_2, w_3$ & 1.4, 3.0, 0.75 \\
            Plan prior matching weight $\beta$  & $5.0 \times 10^{-4}$ \\
            Regularizer weight $\beta_1$  & $1.0 \times 10^{-4}$ \\
            Regularizer weight $\beta_2$  & $1.0 \times 10^{-5}$ \\
            Regularizer weight $\gamma_1$ & $5.0 \times 10^{-3}$ \\
            Regularizer weight $\gamma_2$  & $1.0 \times 10^{-5}$ \\
        \hline
    \end{tabular}
    }
\end{table}

\begin{table}[ht]
    \centering
    \caption{Important hyperparameters (Zero-shot Multi Environment)}
    \label{table: important hyperparameters (Zero-shot Multi Environment)}
    \resizebox{.4\textwidth}{!}{
    \begin{tabular}{ c | c} 
        \hline
            Description & Value \\
        \hline
            Batch Size & 32 \\
            Learning Rate & $1.0 \times 10^{-4}$ \\ 
            Skill Embedding Dimension & 20 \\
            Horizon Length $H$ of Skill & 5 \\
            Magic Scales $w_1, w_2, w_3$ & 1.4, 3.0, 0.75 \\
            Plan prior matching weight $\beta$  & $1.0 \times 10^{-4}$ \\
            Regularizer weight $\beta_1$ & $1.0 \times 10^{-4}$ \\
            Regularizer weight $\beta_2$  & $1.0 \times 10^{-5}$ \\
            Regularizer weight $\gamma_1$ & $5.0 \times 10^{-3}$ \\
            Regularizer weight $\gamma_2$  & $1.0 \times 10^{-5}$ \\
        \hline
    \end{tabular}
    }
\end{table}

\section{Computation Time}
\begin{table}[ht]
  \caption{Training time in hours}\label{tab:computation time}
  \centering
  \resizebox{0.4\textwidth}{!}{
  \begin{tabular}{l l l l}
    \hline
      Environment & LangLfP & HULC & SPIL(ours) \\
    \hline
      D $\rightarrow$ D & 30 & 42 & 43 \\
      ABC $\rightarrow$ D & 102 & 122 & 125 \\
    \hline
  \end{tabular}
  }
\end{table}
\textbf{Hardware and Software}: All of the experiments were performed on a virtual machine with 40 virtual processing units, 356 GB RAM, and two Tesla V100 (16GB) GPUs. The virtual machine is equipped with the Ubuntu-20.04-LTS-focal operating system.
Table \ref{tab:computation time} shows the training time for each model, which was done with 40 epochs for Single Environment (D $\rightarrow$ D) and 30 epochs for Zero-shot Multi Environment (ABC $\rightarrow$ D).

\section{Theoretical Motivation}
\subsection{Continuous Skill Embeddings With Base Skill Priors}
\label{subsec:Continuous Skill Embeddings With Base Skill Priors}
\begin{figure}[h]
    \centering

    \includegraphics[width=0.98\linewidth]{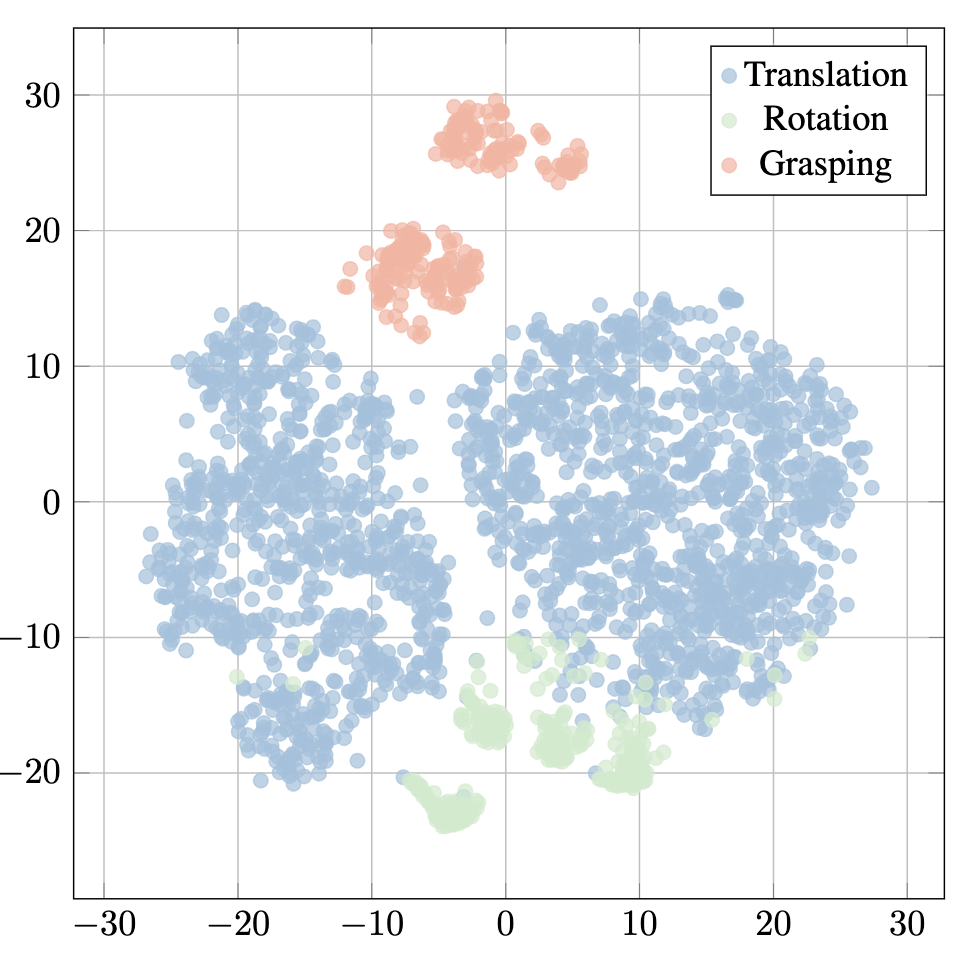}
    \caption{Skill Latent Space}
    \label{fig:example}
\end{figure}

We define $y$ as the indicator for base skills and the base skill distribution in the latent space can be written as $z \sim p(z|y)$. For given action sequence $x$, we employ the approximate variational posterior $q(z|x)$ and $q(y,z|x)$ to estimate the intractable true posterior. Following the VAEs procedure, we measure the Kullback-Leibler (KL) divergence between the true posterior and the posterior approximation to determine the ELBO:
\begin{equation}
    \label{eq:kl_pq_1}
    % \resizebox{0.5\textwidth}{!}{%
    % $
    \begin{split}
        D_{KL}(q(y,z|x) || p(y,z|x))& = \int_y \int_z q(y,z|x) \log \frac{q(y,z|x)}{p(y,z|x)}dzdy \\
            & = - \int_y \int_z q(y,z|x) \log \frac{p(y,z|x)}{q(y,z|x)}dzdy \\
            & = - \int_y \int_z q(y,z|x) \log \frac{p(x,y,z)}{q(z,y|x)}dzdy\\
            & + \log p(x) \\
     \end{split}
     % $%
     % }
\end{equation}
\begin{equation}
    \label{eq:kl_pq_2}
    % \resizebox{0.48\textwidth}{!}{%
    % $
    \begin{split}
        D_{KL}(q(z|x)||p(z|x)) = - \int_z q(z|x) \log \frac{p(z,x)}{q_(z|x)} dz + \log p(x)
    \end{split}
    % $%
    % }
\end{equation}
By combining Equation \ref{eq:kl_pq_1} and Equation \ref{eq:kl_pq_2}, we have:
\begin{equation}
    \label{eq:elbo+kl}
    \begin{split}
        \log p(x) & = \frac{1}{2} \bigg( \overbrace{\int_y \int_z q(y,z|x) \log \frac{p(x,y,z)}{q(z,y|x)p(x)}dzdy}^{\mathcal{L}_1} \\
        & + \overbrace{\int_z q(z|x) \log \frac{p(z,x)}{q(z|x)} dz} ^{\mathcal{L}_2} + D_{KL}(q(y,z|x) || p(y,z|x)) \\
        & + D_{KL}(q(z|x)||p(z|x))\bigg)
    \end{split}
\end{equation}
We focus on the ELBO term $\mathcal{L}_{\textrm {ELBO}} = \frac{1}{2}(\mathcal{L}_1 + \mathcal{L}_2)$:
\begin{equation}
    \begin{split}
        \mathcal{L}_1 & = \int_y \int_z q(y,z|x) \log \frac{p(x,y,z)}{q(z,y|x)}dzdy \\
            & = \int_y \int_z q(z|x,y)q(y|x) \log \frac{p(x|y,z)p(z|y)p(y)}{q(z,y|x)}dzdy \\
            & = \int_y q(y|x) \bigg(\int_z q(z|x,y) \log p(x|y,z) dz \\ 
            & \quad + \int_z q(z|x,y) \log \frac{p(z|y)}{q(z|x,y)} dz \\
            & \quad + \int_z q(z|x,y) \log \frac{p(y)}{q(y|x)} dz \bigg) dy\\
            & = \int_y q(y|x) \bigg(\int_z q(z|x,y) \log p(x|y,z) dz \\ 
            & \quad + \int_z q(z|x,y) \log \frac{p(z|y)}{q(z|x,y)} dz +  \log \frac{p(y)}{q(y|x)} \bigg) dy\\
            % & = \int_y q(y|x) \bigg(\int_z q(z|x,y) \log p(x|y,z) dz \\ 
            % & \quad + \int_z q(z|x,y) \log \frac{p(z|y)}{q(z|x,y)} dz \bigg) dy \\ 
            % & \quad +  \int_y q(y|x) \log \frac{p(y)}{q(y|x)}  dy\\
            & = \int_y q(y|x) \bigg(\int_z q(z|x,y) \log p(x|y,z) dz\\
            & \quad - D_{KL}(q(z|x,y)||p(z|y)) \bigg) dy \\
            & \quad - D_{KL}(q(y|x)||p(y)) \\
    \end{split}
\end{equation}
We define $\boldsymbol{\theta}$ and $\boldsymbol{\phi}$ as parameters for the encoder $q_{\boldsymbol{\phi}}(z|y,x)$ and decoder network $p_{\boldsymbol{\theta}}(x|y,z)$. 
We also define a network $p_{\boldsymbol{\kappa}}(z|y)$ with parameters $\boldsymbol{\kappa}$ for locating the base skills in the latent skill space. In our setups, the variables $x$ and $y$ are conditionally independent given $z$; the variables $z$ and $y$ are also conditionally independent given $x$. Hence, the above equation can be simplified as:
\begin{equation}
    \begin{split}
        \mathcal{L}_1 & = \int_y q(y|x) \bigg(\int_z q_{\boldsymbol{\phi}}(z|x) \log p_{\boldsymbol{\theta}}(x|z) dz \\
                      & \quad - D_{KL}(p_{\boldsymbol{\kappa}}(z|y)||q_{\boldsymbol{\phi}}(z|x)) \bigg) dy - D_{KL}(q(y|x)||p(y)) \\
            & = \int_z q_{\boldsymbol{\phi}}(z|x) \log p_{\boldsymbol{\theta}}(x|z) dz - \int_y q(y|x) D_{KL}(q_{\boldsymbol{\phi}}(z|x)||p_{\boldsymbol{\kappa}}(z|y)) dy \\
            & \quad - D_{KL}(q(y|x)||p(y)) \\
            & = \mathbb{E}_{z \sim q_{\boldsymbol{\phi}}(z|x)} [\log p_{\boldsymbol{\theta}}(x|z)] - \int_y q(y|x) D_{KL}(q_{\boldsymbol{\phi}}(z|x)||p_{\boldsymbol{\kappa}}(z|y)) dy \\
            & \quad - D_{KL}(q(y|x)||p(y)) \\
    \end{split}
\end{equation}
We know the variable $y$ is not continuous and has only three possibilities so it can be computed exactly by marginalizing over these three categorical options. 
\begin{equation}
    \begin{split}
        \mathcal{L}_1 & = \mathbb{E}_{z \sim q_{\boldsymbol{\phi}}(z|x)} [\log p_{\boldsymbol{\theta}}(x|z)] \\
                     & \quad - \sum_{k} q(y=k|x) D_{KL}(q_{\boldsymbol{\phi}}(z|x)||p_{\boldsymbol{\kappa}}(z|y=k)) \\
                     & \quad - D_{KL}(q(y|x)||p(y)) \\
    \end{split}
\end{equation}
In terms of $\mathcal{L}_2$, we have
\begin{equation}
    \mathcal{L}_2 = \mathbb{E}_{z \sim q_{\boldsymbol{\phi}}(z|x)}[\log p_{\boldsymbol{\theta}}(x|z)] - D_{KL} (q_{\boldsymbol{\phi}}(z|x)||p(z)) 
\end{equation}
Then, the total $\mathcal{L}_{\textrm{ELBO}}$ is formalized as:
\begin{equation}
    \begin{split}
    \mathcal{L}_{\textrm{ELBO}} & = \overbrace{\mathbb{E}_{z \sim q_{\boldsymbol{\phi}}(z|x)}[\log p_{\boldsymbol{\theta}}(x|z)]}^{\textrm{reconstruction loss}} - \beta_1 \overbrace{D_{KL} (q_{\boldsymbol{\phi}}(z|x)||p(z))}^{\textrm{regularizer ($\mathcal{L}_{\textrm{reg.}}$)}}\\
    & - \beta_2 \sum_{k} q(y=k|x) \underbrace{D_{KL}(q_{\boldsymbol{\phi}}(z|x)||p_{\boldsymbol{\kappa}}(z|y=k))}_{\textrm{base-skill regularizer ($\mathcal{L}_\textrm{skill}$)}}
    \end{split}\text{,}
\end{equation}

\subsection{Imitation Learning with Base Skill Priors}
\label{appedixsec:Imitation Learning with Base Skill Priors}

The objective of our model is to learn a policy $\pi(x|s_c,s_g)$ conditioned on the current state $s_c$ and the goal state $s_g$ and outputting $x$, a sequence of actions, namely a skill. Since we introduced the base skill concept into our model, the policy $\pi(\cdot)$ should also find the best base skill $y$ for the current observation. We have $\pi(x,y|s_c,s_g)$, where $y$ is the base skill the agent chooses based on the current state and goal state. \\
Inspired by the conditional variational autoencoder (CVAE):
\begin{equation}
    \log p(x|c) \ge \mathbb{E}_{q(z|x,c)}[\log p(x|z,c)] - D_{KL}(q(z|x,c) || p(z|c))
\end{equation}
where c is a symbol to describe a general condition, we would like to extend the above equation by integrating $y$ which indicates the base skill. The evidence we would like to maximize then turns to $p(x,y|c)$. We employ the approximate variational posterior $q(y,z|x,c)$ to approximate the intractable true posterior $p(y,z|x,c)$ where $z$ indicates the skill embeddings in the skill latent space. We intend to find the ELBO by measuring the KL divergence between the true posterior and the posterior approximation.

\begin{equation}
    % \resizebox{0.5\textwidth}{!}{%
    % $
    \begin{split}
        &D_{KL}(q(y,z|x,c) || p(y,z|x,c))  \\
        = & \int_y \int_z q(y,z|x,c) \log \frac{q(y,z|x,c)}{p(y,z|x,c)}dzdy \\
        = & - \int_y \int_z q(y,z|x,c) \log \frac{p(y,z|x,c)}{q(y,z|x,c)}dzdy \\
        = & - \int_y \int_z q(y,z|x,c) \log \frac{p(x,y,z|c)}{q(z,y|x,c)}dzdy + \log p(x|c) \\
    \end{split}
%     $%
% }
\end{equation}

We focus on the ELBO term:
\begin{equation}
    % \resizebox{0.5\textwidth}{!}{%
    % $
    \begin{split}
        \mathcal{L} & = \int_y \int_z q(y,z|x,c) \log \frac{p(x,y,z|c)}{q(z,y|x,c)}dzdy \\
                    & = \int_y \int_z q(z|x,y,c)q(y|x,c) \log \frac{p(x|y,z,c)p(z|y,c)p(y|c)}{q(z,y|x,c)} dz dy \\
                    & = \int_y q(y|x,c)\bigg(\int_z q(z|x,y,c) \log p(x|y,z,c) dz \\
                    & \quad + \int_z q(z|x,y,c) \log \frac{p(z|y,c)}{q(z|x,c)} dy + \log \frac{p(y|c)}{q(y|x,c)}\bigg) \\
                    & = \int_y q(y|x,c) \bigg( \int_z q(z|x,y,c) \log p(x|y,z,c) dz \\ 
                    & \quad - D_{KL} (q(z|x,y,c)||p(z|y,c)) \bigg) dy - D_{KL} (q(y|x,c)||p(y))
    \end{split}
%     $%
% }
\end{equation}
To have a clear explanation, we examine each element in the equation mentioned above.
\begin{itemize}
    \item variable $x,y,z,c$:
        \begin{itemize}
            \item $x$: action sequence (skill) the agent chooses
            \item $y$: base skill priors
            \item $z$: skill embeddings in the latent skill space
            \item $c$: a combination of the current state and the goal state $(s_c,s_g)$
        \end{itemize}
    \item $q(y|x,c)$: It corresponds to the base skill labeler part in our SPIL model. We define this network with parameters $\boldsymbol{\omega}$ and simplify it as $q_{\boldsymbol{\omega}}(y|c)$ by pointing out $x$. 
    \item $q(z|x,y,c)$: It refers to the encoder network $f_{\boldsymbol{\Phi}}$ plus the skill embedding selector network $f_{\boldsymbol{\lambda}}$, taking $c$ as input in our settings. It can be written as $q_{\boldsymbol{\Phi}, \boldsymbol{\lambda}}(z|c)$, pointing out $x,y$.
    \item $p(x|y,z,c)$: It is the skill generator network $f_{\boldsymbol{\theta}}$ with parameters $\boldsymbol{\theta}$. This network only takes $z,c$ as input in our setting and we consider $x$ and $y$ to be conditionally independent given $z,c$. It can then be formalized as $p(x|z,c)$. Note that the parameters of this network are pretrained and frozen during the training process. 
    \item $p(z|y,c)$: It is the base skill prior locater $f_{\boldsymbol{\kappa}}$ with parameter $\boldsymbol{\kappa}$. We assume $z$ and $c$ are conditionally independent given $y$ so that we have $p_{\boldsymbol{\kappa}}(z|y)$. Note that the parameters of this network are frozen during the training. 
    \item $p(y)$: It is the prior distribution for base skills $y$ which is drawn from a categorical distribution. 

\end{itemize}
Based on the above analysis, the whole equation can be simplified as follows:
\begin{equation}   
    \begin{split}
    \mathcal{L} & =\int_y q_{\boldsymbol{\omega}}(y|c) \bigg( \int_z q_{\boldsymbol{\Phi}, \boldsymbol{\lambda}}(z|c) \log p_{\boldsymbol{\theta}}(x|z,c) dz \\ 
                & \quad - D_{KL}(q_{\boldsymbol{\Phi}, \boldsymbol{\lambda}}(z|c)||p_{\boldsymbol{\kappa}}(z|y))\bigg) dy - D_{KL}(q(y|c)||p(y)) \\
                & = \int_z q_{\boldsymbol{\Phi}, \boldsymbol{\lambda}}(z|c) \log p_{\boldsymbol{\theta}}(x|z,c) dz \\
                & \quad - \int_y q_{\boldsymbol{\omega}}(y|c) D_{KL}(q_{\boldsymbol{\Phi}, \boldsymbol{\lambda}}(z|x,c)||p_{\boldsymbol{\kappa}}(z|y)) dy \\
                & \quad - D_{KL}(q_{\boldsymbol{\omega}}(y|c)||p(y)) \\
                & = \mathbb{E}_{z \sim q_{\boldsymbol{\Phi}, \boldsymbol{\lambda}}(z|c)}\log p_{\boldsymbol{\theta}}(x|z,c) \\
                & \quad - \sum_{k} q_{\boldsymbol{\omega}}(y=k|c) D_{KL}(q_{\boldsymbol{\Phi}, \boldsymbol{\lambda}}(z|c)||p_{\boldsymbol{\kappa}}(z|y)) \\ 
                & \quad - D_{KL}(q_{\boldsymbol{\omega}}(y|c)||p(y))
    \end{split}
\end{equation}
By introducing two weights $\gamma_1$ and $\gamma_2$ for the regularization terms, we have 
\begin{equation}
    \begin{split}
        \mathcal{L} & = \overbrace{\mathbb{E}_{z \sim q_{\boldsymbol{\Phi}, \boldsymbol{\lambda}}(x,c)}\log p_{\boldsymbol{\theta}}(x|z,c)}^{\textrm{Reconstruction loss}} \\ 
        & - \gamma_1 \sum_{k} q_{\boldsymbol{\omega}}(y=k|c) \overbrace{D_{KL}(q_{\boldsymbol{\Phi}, \boldsymbol{\lambda}}(z|x,c)||p_{\boldsymbol{\kappa}}(z|y))}^{\textrm{Base skill regularizer ($\mathcal{L}_{\textrm{skill}}$)}}\\
        & - \gamma_2 \overbrace{D_{KL}(q_{\boldsymbol{\omega}}(y|c)||p(y))}^{\textrm{Categorical regularizer ($\mathcal{L}_{\textrm{cat.}}$)}}
    \end{split}
\end{equation}
Here, we use Huber loss as the metric for reconstructive loss.
% \begin{equation}
%     \label{eq:loss function of spil}
%     \resizebox{0.5\textwidth}{!}{%
%     $
%     \begin{split}
%         \mathcal{L} & = \mathcal{L}_{huber}(x, \hat{x}) + \gamma_1 \sum_{k} q_{\boldsymbol{\boldsymbol{\lambda}}}(y=k|c) D_{KL}(q_{\boldsymbol{\phi}}(z|x,c)||p_{\boldsymbol{\kappa}}(z|y))\\ 
%         & + \gamma_2 D_{KL}(q_{\boldsymbol{\lambda}}(y|c)||p(y))
%     \end{split}
%     $%
%     }
% \end{equation}
Intuitively, the base skill regularizer is used to regularize a skill embedding, depending on its base skill categorial. The categorial regularizer aims to regularize the base skill classification based on the prior categorical distribution of $y$.
